# Supplementary material for: An increase in black hole activity in galaxies with kinematically misaligned gas
Source: arXiv:2301.07155 source file (2023-01-17)
Supplement: Supplementary file 1 [file Raimundo_SI.pdf]

## **Supplementary information**

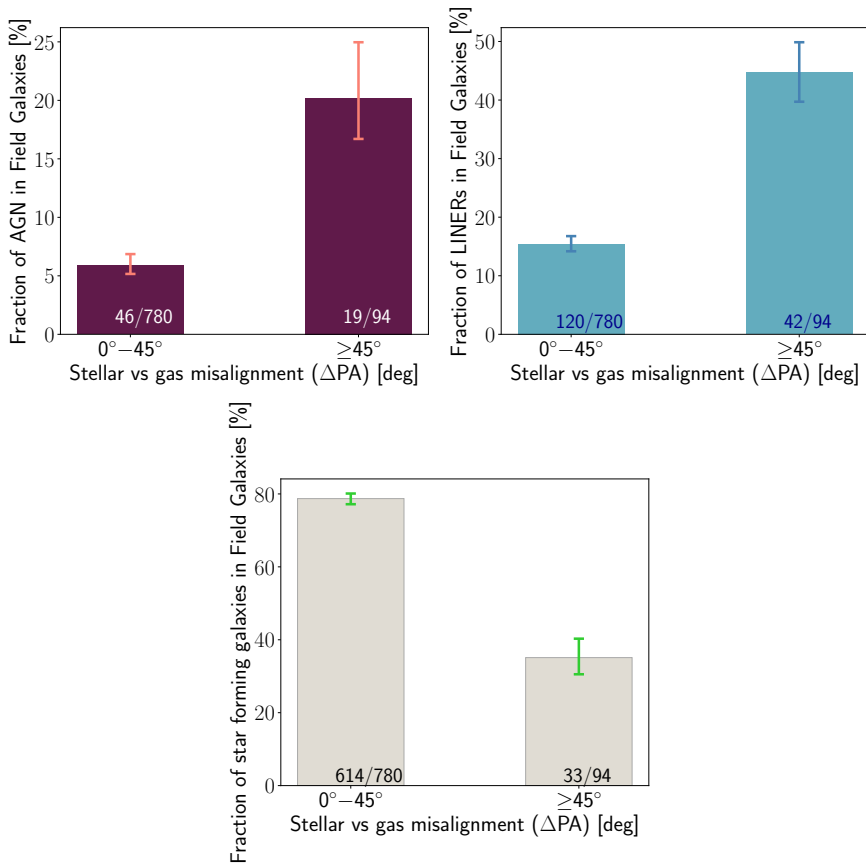

**Fig. 1:** Field/group galaxies. The two top panels in the figure show the fraction of Active Galactic Nuclei (AGN - top left panel) and the fraction of Low Ionization Nuclear Emission Line Regions (LINERs - top right panel) in the sample of 1091 galaxies with measured  $\Delta PA$  and excitation mechanism. The bottom panel shows the fraction of Star Forming galaxies. The galaxies are divided according to the angle difference between the stellar and ionised gas kinematic axis ( $\Delta PA = |PA_{\text{star}} - PA_{\text{gas}}|$ ). Large kinematic misalignment between the stellar and gas rotation is a clear signature of an external accretion event, such as a galaxy merger or the accretion of gas from the immediate external environment of a galaxy. The two histogram bars show aligned ( $0^\circ < \Delta PA < 45^\circ$ ) and misaligned ( $45^\circ \leq \Delta PA \leq 180^\circ$ ) galaxies with error bars that indicate the 68% confidence interval. The numbers at the base of the histogram bars show the number of AGN, LINERs or star forming galaxies compared with the total number of galaxies in each bin. This figure shows the field/group galaxies which drive the relation for the total population.

**Table 1:** Table containing a summary of the main results for the sample of 1310 galaxies with measured stellar and gas kinematic angles. Truncated for visualization purposes. A full version of this table is provided as part of the supplementary information.

| catid  | ra_obj<br>[deg]<br>[1] | dec_obj<br>[deg]<br>[3] | z_spec<br>[4] | PA_s<br>[deg]<br>[5] | PA_s_e<br>[ $\pm$ deg]<br>[6] | PA_g<br>[deg]<br>[7] | PA_g_e<br>[ $\pm$ deg]<br>[8] | $\Delta$ PA<br>[deg]<br>[9] | $\Delta$ PA_e<br>[ $\pm$ deg]<br>[10] | flag<br>[11] | f_AGN<br>[12] | type<br>[13] | mstar<br>[log M <sub>⊙</sub> ]<br>[14] |
|--------|------------------------|-------------------------|---------------|----------------------|-------------------------------|----------------------|-------------------------------|-----------------------------|---------------------------------------|--------------|---------------|--------------|----------------------------------------|
| 100162 | 185.7931               | 0.9349                  | 0.0258        | 48.3                 | 11.6                          | 52.3                 | 0.5                           | 4.0                         | 12.1                                  | s            |               | 3.0          | 9.15                                   |
| 100192 | 185.9277               | 0.9622                  | 0.0241        | 230.3                | 7.0                           | 223.2                | 0.5                           | 7.0                         | 7.5                                   | s            |               | 3.0          | 9.33                                   |
| 105447 | 211.7731               | 0.8564                  | 0.0487        | 219.2                | 2.5                           | 221.2                | 1.5                           | 2.0                         | 4.0                                   | 1            |               | 1.5          | 10.11                                  |
| 105519 | 212.3402               | 1.0277                  | 0.0577        | 49.3                 | 2.5                           | 264.5                | 14.1                          | 144.8                       | 16.6                                  |              |               | 1.0          | 10.34                                  |
| 105597 | 212.7404               | 1.0357                  | 0.0254        | 281.6                | 1.5                           | 283.6                | 0.5                           | 2.0                         | 2.0                                   | s            |               | 2.0          | 10.41                                  |
| 105738 | 213.2469               | 0.9212                  | 0.0529        | 311.7                | 4.5                           | 329.8                | 0.5                           | 18.1                        | 5.0                                   | a            |               | 1.0          | 10.50                                  |
| 106016 | 214.4182               | 0.9202                  | 0.0535        | 49.3                 | 4.5                           | 49.3                 | 2.5                           | 0.0                         | 7.0                                   | 1            |               | 1.0          | 10.23                                  |
| 106042 | 214.5621               | 0.8911                  | 0.0260        | 277.5                | 2.5                           | 271.5                | 0.5                           | 6.0                         | 3.0                                   | s            |               | 3.0          | 10.14                                  |
| 106047 | 214.5697               | 0.9863                  | 0.0534        | 194.1                | 7.5                           | 214.2                | 0.5                           | 20.1                        | 8.0                                   | s            |               | 1.5          | 10.14                                  |
| 106331 | 215.5132               | 0.8621                  | 0.0360        | 335.9                | 6.5                           | 340.9                | 0.5                           | 5.0                         | 7.0                                   | s            |               | 3.0          | 9.61                                   |

Labels: [1] Catalogue ID from the SAMI survey DR3. [2] Right ascension. [3] Declination. [4] Spectroscopic redshift. [5] Principal stellar kinematic axis ( $PA_{\text{stellar}}$ ). [6]  $3\sigma$  uncertainty in  $PA_{\text{stellar}}$ . [7] Principal gas kinematic axis ( $PA_{\text{gas}}$ ). [8]  $3\sigma$  uncertainty in  $PA_{\text{gas}}$ . [9] Difference in stellar-gas kinematic angles ( $\Delta PA = |PA_{\text{stellar}} - PA_{\text{gas}}|$ ). [10]  $3\sigma$  uncertainty in  $\Delta PA$ . [11] Flag for excitation mechanism (s - star-forming galaxy; l - LINER; a- AGN). [12] Flag for AGN detection from broad lines (bl), X-ray catalogue (x), radio catalogue (r) or infrared WISE catalogue (w). [13] Morphological type as in the SAMI survey classification (see text). [14] Stellar mass. Columns 1 - 4 and 13 - 14 were taken directly from the SAMI survey results and shown here for reference.

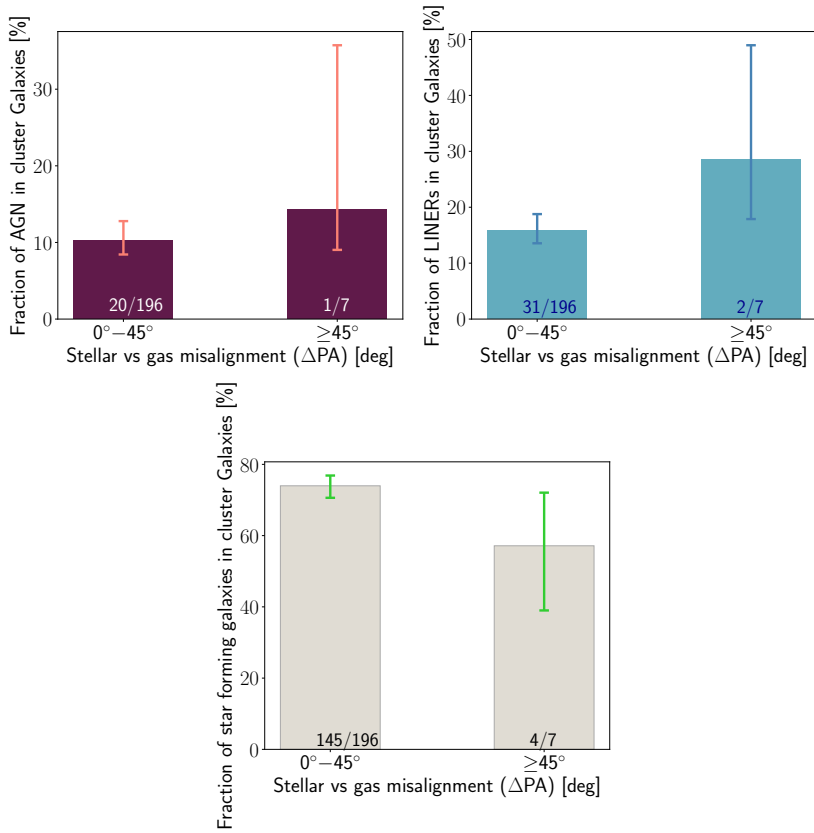**Fig. 2:** Similar to Fig. 1 but showing only the cluster galaxies.

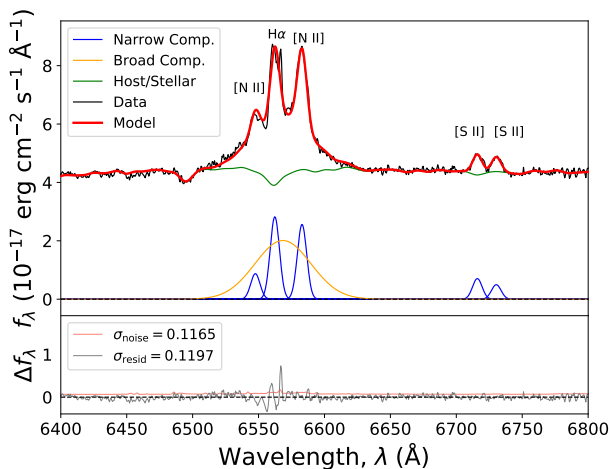

**Fig. 3:** Example of a SAMI galaxy where a nuclear H $\alpha$  broad emission line has been detected. The top panel of the figure shows the nuclear spectrum in black and the result of the spectral fitting with the BADASS algorithm in red, with the x-axis being the rest-frame wavelength and the y-axis the measured flux. The different components of the fit are shown in green (the host galaxy component), blue (narrow emission lines) and orange (broad emission line). The noise level (orange horizontal line) and fit residuals (grey line) are shown in the bottom panel.

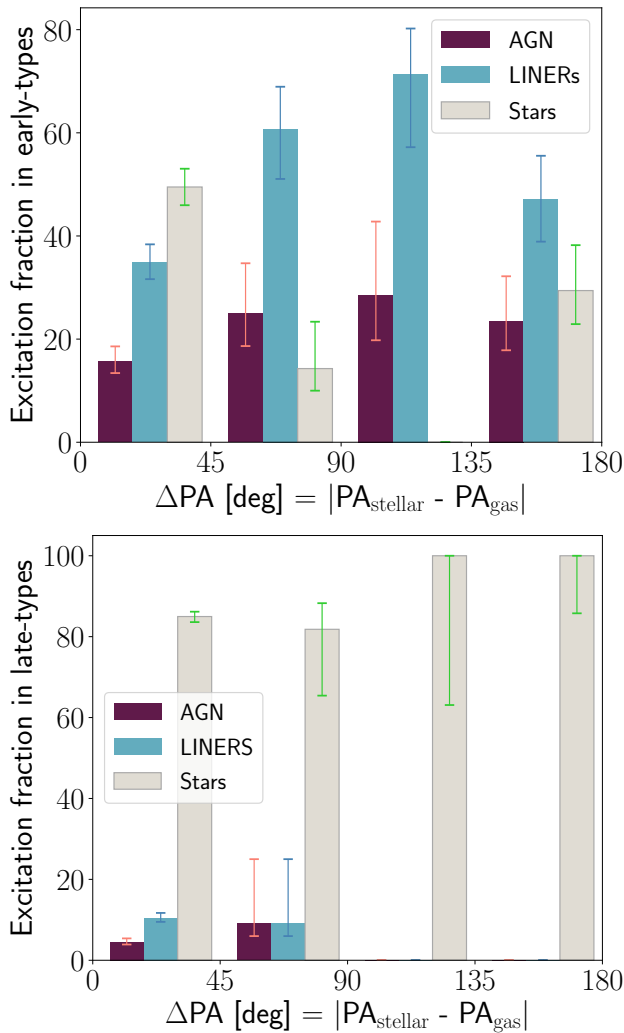

**Fig. 4:** Percentage of galaxies with different excitation mechanisms divided per interval of misalignment angle ( $\Delta\text{PA}$ ) and as a function of morphology (early-type galaxies on the left and late-type galaxies on the right). Due to the low number of galaxies the histogram has been divided into  $\Delta\text{PA} = 45^\circ$  bins which corresponds to a minimum of 17 total galaxies per bin. The histogram shows four bins:  $0^\circ \leq \Delta\text{PA} < 45^\circ$ ,  $45^\circ \leq \Delta\text{PA} < 90^\circ$ ,  $90^\circ \leq \Delta\text{PA} < 135^\circ$  and  $135^\circ \leq \Delta\text{PA} \leq 180^\circ$ . The errors bars correspond to the 68% confidence intervals using a beta distribution quantile technique (see main text for references). The error bars for the last two bins show the one-sided confidence interval because the value of those histogram bars is 100%.

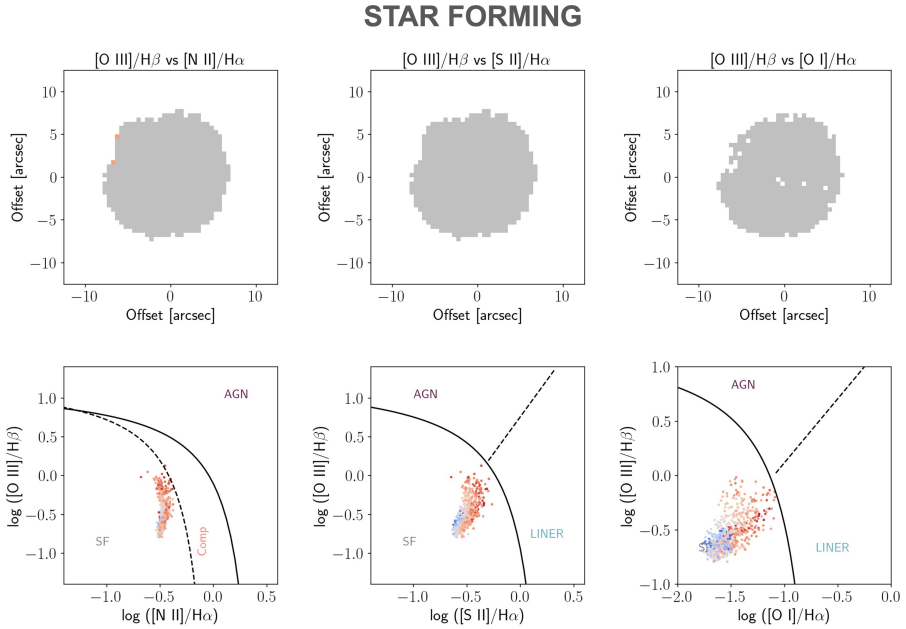

**Fig. 5:** Illustration of the line diagnostics used. The figure shows an example of a galaxy classified as star-forming. The figure shows the BPT analysis used to identify the excitation mechanisms: The three top panels show the galaxy spatial maps colour-coded by dominant excitation mechanism, purple for AGN, salmon for composite, grey for star formation and blue for LINER. Bottom panels show the BPT diagrams for each spaxel in the image, colour-coded as a function of distance from centre of the galaxy (shown as position (0,0) in the top panels). Blue symbols correspond to spaxels closest to the nucleus, red symbols to spaxels further away from the nucleus, with the range of colours calibrated for each individual galaxy. For example, the bluest point for each galaxy will be the spaxel with detected emission that is closest to its nucleus. That could be the central spaxel (distance = 0) or a spaxel that is further away from the nucleus if no emission is detected in the central spaxels. The solid and dashed lines are the classification boundaries from [62]. Each column refers for a specific line ratio, from left to right:  $[\text{O III}]/\text{H}\beta$  vs  $[\text{N II}]/\text{H}\alpha$ ,  $[\text{O III}]/\text{H}\beta$  vs  $[\text{S II}]/\text{H}\alpha$  and  $[\text{O III}]/\text{H}\beta$  vs  $[\text{O I}]/\text{H}\alpha$ . The labels in the bottom row refer to the excitation classification in each region of the diagrams: AGN, LINER, SF (star-forming galaxies) or Comp (composite regions).
